# Supplementary material for: Software Entity Recognition with Noise-Robust Learning
Source: arXiv:2308.10564 source file (2023-08-21)
Supplement: Supplementary file 1 [file appendix.tex]

\section{Appendix}
% NO APPENDIX FOR SE CONFERENCES
